# Supplementary material for: Micro Visualizations on a Smartwatch: Assessing Reading Performance While Walking
Source: arXiv:2407.17893 source file (2024-07-25)
Supplement: Supplementary file 1 [file appendices.tex]

\begin{figure*}[t!]
    \centering
    \vspace{-1em}
    \subfloat[]{
        \includegraphics[width=0.32\linewidth]{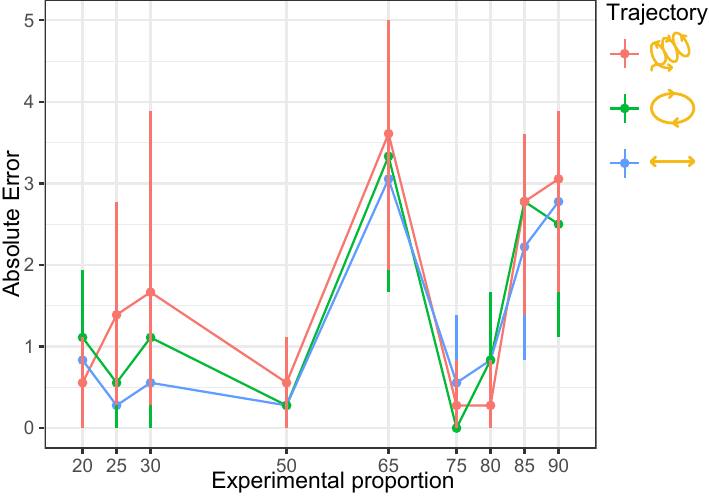}
        \label{fig:abs_erorr_S1}
    }
    \subfloat[]{
        \includegraphics[width=0.305\linewidth]{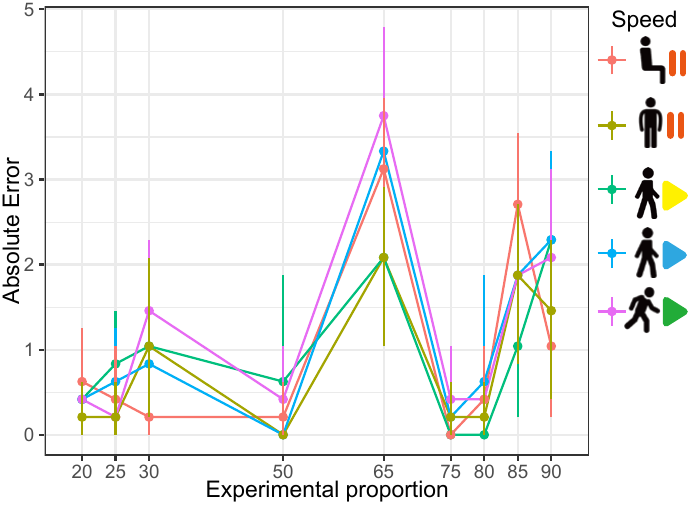}
        \label{fig:abs_error_S2}
    }
    \vspace{-1em}
    \caption{Absolute error for the proportion estimation task per percentage for the three walking trajectories. (a) Results from Study~1: \lineIcon\ line, \circularIcon\ circular, and \infinityIcon\ infinity trajectory. (b) Results from Study~2: \standIcon\ Standing, \sitIcon\ Sitting, \slowWalkIcon km/h, \fastWalkIcon km/h, \slowJogIcon km/h.}
    \label{fig:results_abs_true_error}
\end{figure*}

%%% table for task difficulty, confidence level, and efforts demanding 
\begin{table*}[h]
    \centering
    \caption{Participants' ratings in Study 1: (a) confidence in response correctness, (b) task difficulty rating, (c) mental effort, and (d) physical effort, with median (MED), average (AVG) and standard deviation (SD). \lineIcon: line trajectory, \circularIcon: circular trajectory, \infinityIcon: infinity trajectory}
    %{with 1: Very easy; Not confident at all; Not demanding at all and 7: Very difficult; Very confident; Very demanding}.
      \label{fig:results_time}
    \captionsetup{justification=centering}
    \footnotesize

    \subfloat[Confidence in response correctness per trajectory.\\ 1: not at all confident, 7: very confident\label{tab:study1_confidence}]{
        
        \begin{tabular}{c
                    c
                    c
                    c
                    c
                    c
                    c
                    c
                    |c
                    |c
                    |c}
        \toprule
        & 1 & 2 & 3 & 4 & 5 & 6 & 7 & MED & AVG & SD \\
        \midrule
        \lineIcon\
        & \databar[isot]{0} & \databar[isot]{0} & \databar[isot]{1} & \databar[isot]{5} & \databar[isot]{5} & \databar[isot]{7} & \databar[isot]{0}
        & 5
        & 5.00
        & 0.97\\
        
        \midrule
        
        \circularIcon\
        & \databar[isot]{0} & \databar[isot]{0} & \databar[isot]{2} & \databar[isot]{2} & \databar[isot]{7} & \databar[isot]{6} & \databar[isot]{1}
        & 5
        & 5.11
        & 1.08\\
        
        \midrule

        \infinityIcon\
        & \databar[isot]{0} & \databar[isot]{1} & \databar[isot]{2} & \databar[isot]{4} & \databar[isot]{5} & \databar[isot]{5} & \databar[isot]{1}
        & 5
        & 4.78
        & 1.31\\
        
        \bottomrule
        \end{tabular}    
    }
    %\hfill
    \subfloat[Task difficulty rating per trajectory. \\
    1: not at all difficult, 7: very difficult\label{tab:study1_difficulty}]{
        
        \begin{tabular}{c@{\quad}
                    c
                    c
                    c
                    c
                    c
                    c
                    c
                    |c
                    |c
                    |c}
        \toprule
        & 1 & 2 & 3 & 4 & 5 & 6 & 7 & MED & AVG & SD \\
        \midrule
        \lineIcon\
        & \databar[isot]{0} & \databar[isot]{4} & \databar[isot]{5} & \databar[isot]{3} & \databar[isot]{5} & \databar[isot]{1} & \databar[isot]{0}
        & 3.5
        & 3.67
        & 1.28\\
        
        \midrule
        
        \circularIcon\
        & \databar[isot]{0} & \databar[isot]{6} & \databar[isot]{4} & \databar[isot]{4} & \databar[isot]{3} & \databar[isot]{1} & \databar[isot]{0}
        & 3
        & 3.39
        & 1.29\\
        
        \midrule

        \infinityIcon\
        & \databar[isot]{0} & \databar[isot]{3} & \databar[isot]{4} & \databar[isot]{3} & \databar[isot]{7} & \databar[isot]{1} & \databar[isot]{0}
        & 4
        & 3.94
        & 1.26\\
        
        \bottomrule
        \end{tabular}    
    }
    %\vspace{0.3cm}
    \\
    \subfloat[Mental effort per trajectory. \\
    1: not at all demanding, 7: very demanding\label{tab:study1_mentalLoad}]{
        
        \begin{tabular}{c@{\quad}
                    c
                    c
                    c
                    c
                    c
                    c
                    c
                    |c
                    |c
                    |c}
        \toprule
        & 1 & 2 & 3 & 4 & 5 & 6 & 7 & MED & AVG & SD \\
        \midrule
         \lineIcon\
        & \databar[isot]{1} & \databar[isot]{2} & \databar[isot]{5} & \databar[isot]{6} & \databar[isot]{2} & \databar[isot]{2} & \databar[isot]{0}
        & 4
        & 3.67
        & 1.33\\
        
        \midrule
        
        \circularIcon\
        & \databar[isot]{0} & \databar[isot]{3} & \databar[isot]{6} & \databar[isot]{5} & \databar[isot]{1} & \databar[isot]{3} & \databar[isot]{0}
        & 3.5
        & 3.72
        & 1.32\\
        
        \midrule

        \infinityIcon\
        & \databar[isot]{0} & \databar[isot]{1} & \databar[isot]{5} & \databar[isot]{4} & \databar[isot]{4} & \databar[isot]{4} & \databar[isot]{0}
        & 4
        & 4.28
        & 1.27\\
        
        \bottomrule
        \end{tabular}    
    }
     %\hfill
    \subfloat[Physical effort per trajectory. \\
    1: not at all demanding, 7: very demanding\label{tab:study1_physicalLoad}]{
        
        \begin{tabular}{c@{\quad}
                    c
                    c
                    c
                    c
                    c
                    c
                    c
                    |c
                    |c
                    |c}
        \toprule
        & 1 & 2 & 3 & 4 & 5 & 6 & 7 & MED & AVG & SD \\
        \midrule
        \lineIcon\
        & \databar[isot]{10} & \databar[isot]{4} & \databar[isot]{2} & \databar[isot]{1} & \databar[isot]{1} & \databar[isot]{0} & \databar[isot]{0}
        & 1
        & 1.83
        & 1.20\\
        
        \midrule
        
        \circularIcon\
        & \databar[isot]{6} & \databar[isot]{9} & \databar[isot]{1} & \databar[isot]{0} & \databar[isot]{1} & \databar[isot]{1} & \databar[isot]{0}
        & 2
        & 2.11
        & 1.37\\
        
        \midrule

        \infinityIcon\
        & \databar[isot]{7} & \databar[isot]{6} & \databar[isot]{3} & \databar[isot]{1} & \databar[isot]{0} & \databar[isot]{1} & \databar[isot]{0}
        & 2
        & 2.11
        & 1.32\\
        
        \bottomrule
        \end{tabular}    
    }
    \label{tab:study1_questionnaires}

\end{table*}

%%% table for task difficulty, confidence level, and efforts demanding 
\begin{table*}
    \centering
    \captionsetup{justification=centering}
    \footnotesize
    \caption{Participants' ratings in Study 2: (a) confidence in response correctness, (b) task difficulty rating, (c) mental effort, and (d) physical effort, with median (MED), average (AVG) and standard deviation (SD). \\
    \standIcon: Standing (baseline), \sitIcon: Sitting (baseline), \slowWalkIcon: Slow walking at 2km/h, \fastWalkIcon: Fast walking at 4km/h, \slowJogIcon: Slow jogging at 6km/h.}
    \label{tab:study2_questionnaires}
    \subfloat[Confidence in response correctness per condition.\\ 1: not at all confident, 7: very confident\label{tab:study2_confidence}]{
        
        \begin{tabular}{c
                    c
                    c
                    c
                    c
                    c
                    c
                    c
                    |c
                    |c
                    |c}
        \toprule
        & 1 & 2 & 3 & 4 & 5 & 6 & 7 & MED & AVG & SD \\
        \midrule
        \standIcon\
        & \databar[isoorange]{0} & \databar[isoorange]{2} & \databar[isoorange]{2} & \databar[isoorange]{4} & \databar[isoorange]{1} & \databar[isoorange]{13} & \databar[isoorange]{2}
        & 6
        & 5.13
        & 1.48\\
        
        \midrule
        
        \sitIcon\
        & \databar[isoorange]{1} & \databar[isoorange]{1} & \databar[isoorange]{3} & \databar[isoorange]{3} & \databar[isoorange]{2} & \databar[isoorange]{9} & \databar[isoorange]{5}
        & 6
        & 5.13
        & 1.73\\
        
        \midrule

        \slowWalkIcon\
        & \databar[isoyellow]{0} & \databar[isoyellow]{0} & \databar[isoyellow]{2} & \databar[isoyellow]{3} & \databar[isoyellow]{6} & \databar[isoyellow]{9} & \databar[isoyellow]{4}
        & 6
        & 5.42
        & 1.18\\
        
        \midrule

        \fastWalkIcon\
        & \databar[isoblue]{0} & \databar[isoblue]{1} & \databar[isoblue]{2} & \databar[isoblue]{1} & \databar[isoblue]{8} & \databar[isoblue]{9} & \databar[isoblue]{3}
        & 6
        & 5.34
        & 1.27\\
        
        \midrule

        \slowJogIcon\
        & \databar[isogreen]{0} & \databar[isogreen]{3} & \databar[isogreen]{2} & \databar[isogreen]{4} & \databar[isogreen]{8} & \databar[isogreen]{6} & \databar[isogreen]{1}
        & 5
        & 4.63
        & 1.41\\
        
        \bottomrule
        \end{tabular}    
    }
    %\hfill
    \subfloat[Task difficulty rating per condition. \\
    1: not at all difficult, 7: very difficult\label{tab:study2_difficulty}]{
        
        \begin{tabular}{c@{\quad}
                    c
                    c
                    c
                    c
                    c
                    c
                    c
                    |c
                    |c
                    |c}
        \toprule
        & 1 & 2 & 3 & 4 & 5 & 6 & 7 & MED & AVG & SD \\
        \midrule
        \standIcon\
        & \databar[isoorange]{14} & \databar[isoorange]{7} & \databar[isoorange]{3} & \databar[isoorange]{0} & \databar[isoorange]{0} & \databar[isoorange]{0} & \databar[isoorange]{0}
        & 1
        & 1.54
        & 0.72\\
        
        \midrule
        
        \sitIcon\
        & \databar[isoorange]{13} & \databar[isoorange]{8} & \databar[isoorange]{2} & \databar[isoorange]{1} & \databar[isoorange]{0} & \databar[isoorange]{0} & \databar[isoorange]{0}
        & 1
        & 1.63
        & 0.82\\
        
        \midrule

        \slowWalkIcon\
        & \databar[isoyellow]{6} & \databar[isoyellow]{13} & \databar[isoyellow]{5} & \databar[isoyellow]{0} & \databar[isoyellow]{0} & \databar[isoyellow]{0} & \databar[isoyellow]{0}
        & 2
        & 1.96
        & 0.69\\
        
        \midrule

        \fastWalkIcon\
        & \databar[isoblue]{3} & \databar[isoblue]{17} & \databar[isoblue]{1} & \databar[isoblue]{2} & \databar[isoblue]{1} & \databar[isoblue]{0} & \databar[isoblue]{0}
        & 2
        & 2.21
        & 0.93\\
        
        \midrule

        \slowJogIcon\
        & \databar[isogreen]{1} & \databar[isogreen]{5} & \databar[isogreen]{9} & \databar[isogreen]{4} & \databar[isogreen]{3} & \databar[isogreen]{2} & \databar[isogreen]{0}
        & 3
        & 3.38
        & 1.31\\
        
        \bottomrule
        \end{tabular}    
    }
    %\vspace{0.3cm}
    \\
    \subfloat[Mental effort per condition. \\
    1: not at all demanding, 7: very demanding \label{tab:study2_mentalLoad}]{
        
        \begin{tabular}{c@{\quad}
                    c
                    c
                    c
                    c
                    c
                    c
                    c
                    |c
                    |c
                    |c}
        \toprule
        & 1 & 2 & 3 & 4 & 5 & 6 & 7 & MED & AVG & SD \\
        \midrule
        \standIcon\
        & \databar[isoorange]{6} & \databar[isoorange]{14} & \databar[isoorange]{4} & \databar[isoorange]{0} & \databar[isoorange]{0} & \databar[isoorange]{0} & \databar[isoorange]{0}
        & 2
        & 1.92
        & 0.65\\
        
        \midrule
        
        \sitIcon\
        & \databar[isoorange]{9} & \databar[isoorange]{11} & \databar[isoorange]{2} & \databar[isoorange]{1} & \databar[isoorange]{1} & \databar[isoorange]{0} & \databar[isoorange]{0}
        & 2
        & 1.92
        & 1.02\\
        
        \midrule

        \slowWalkIcon\
        & \databar[isoyellow]{6} & \databar[isoyellow]{10} & \databar[isoyellow]{6} & \databar[isoyellow]{2} & \databar[isoyellow]{0} & \databar[isoyellow]{0} & \databar[isoyellow]{0}
        & 2
        & 2.22
        & 0.92\\
        
        \midrule

        \fastWalkIcon\
        & \databar[isoblue]{3} & \databar[isoblue]{17} & \databar[isoblue]{4} & \databar[isoblue]{0} & \databar[isoblue]{0} & \databar[isoblue]{0} & \databar[isoblue]{0}
        & 2
        & 2.04
        & 0.55\\
        
        \midrule

        \slowJogIcon\
        & \databar[isogreen]{3} & \databar[isogreen]{10} & \databar[isogreen]{4} & \databar[isogreen]{5} & \databar[isogreen]{0} & \databar[isogreen]{2} & \databar[isogreen]{0}
        & 2
        & 2.79
        & 1.38\\
        
        \bottomrule
        \end{tabular}    
    }
    %\hfill
    \subfloat[Physical effort per condition. \\
    1: not at all demanding, 7: very demanding\label{tab:study2_physicalLoad}]{
        
        \begin{tabular}{c@{\quad}
                    c
                    c
                    c
                    c
                    c
                    c
                    c
                    |c
                    |c
                    |c}
        \toprule
        & 1 & 2 & 3 & 4 & 5 & 6 & 7 & MED & AVG & SD \\
        \midrule
        \standIcon\
        & \databar[isoorange]{20} & \databar[isoorange]{14} & \databar[isoorange]{0} & \databar[isoorange]{0} & \databar[isoorange]{0} & \databar[isoorange]{0} & \databar[isoorange]{0}
        & 1
        & 1.17
        & 0.38\\
        
        \midrule
        
        \sitIcon\
        & \databar[isoorange]{23} & \databar[isoorange]{1} & \databar[isoorange]{0} & \databar[isoorange]{0} & \databar[isoorange]{0} & \databar[isoorange]{0} & \databar[isoorange]{0}
        & 1
        & 1.04
        & 0.20\\
        
        \midrule

        \slowWalkIcon\
        & \databar[isoyellow]{15} & \databar[isoyellow]{8} & \databar[isoyellow]{1} & \databar[isoyellow]{0} & \databar[isoyellow]{0} & \databar[isoyellow]{0} & \databar[isoyellow]{0}
        & 1
        & 1.42
        & 0.58\\
        
        \midrule

        \fastWalkIcon\
        & \databar[isoblue]{9} & \databar[isoblue]{10} & \databar[isoblue]{4} & \databar[isoblue]{1} & \databar[isoblue]{0} & \databar[isoblue]{0} & \databar[isoblue]{0}
        & 2
        & 1.88
        & 0.85\\
        
        \midrule

        \slowJogIcon\
        & \databar[isogreen]{3} & \databar[isogreen]{2} & \databar[isogreen]{8} & \databar[isogreen]{6} & \databar[isogreen]{5} & \databar[isogreen]{0} & \databar[isogreen]{0}
        & 3
        & 3.33
        & 1.27\\
        
        \bottomrule
        \end{tabular}    
    }
\end{table*}

% measurements Study~1
\setlength{\picturewidth}{.45\linewidth}
\setlength{\pictureheight}{1.65cm}
\setlength{\meanfigwidth}{.1\linewidth}
\setlength{\meanfigheight}{1.3cm}
\setlength{\difffigwidth}{.2\linewidth}
\setlength{\difffigheight}{1.4cm}
\begin{table*}[t!]
   
\centering
    \caption{A copy of Table 2 in the paper including the pairwise differences. Means (top) and pairwise differences (bottom) of the reading performance measurements for Study~1: response time (Row 1), fitness data comparison accuracy (Row 2), proportion estimation accuracy (Row 3). Error bars represent 95\% Bootstrap confidence intervals (CIs) in black, adjusted for three pairwise comparisons with Bonferroni correction (in red).\\
    \small\lineIcon\ line trajectory, \circularIcon\ circular trajectory, \infinityIcon\ infinity trajectory
    \vspace{-0.3cm}\label{tab:study01_measurements-extended}}
    \scriptsize
    \centering
    \fontsize{5.1}{5.3}\selectfont
    \begin{tabular}
    {@{}p{1.4\picturewidth}@{}%for the 1st image
    @{}r@{~}%for writing the average
    @{}p{1cm}@{}%for writing the CI
    % @{}p{1.8\picturewidth}@{}%for the 2nd image
    % @{}r@{~}%for the average
    % @{}p{0.8cm}@{}%for writing the CI
    }
    %%%%%%%% Title row: response time %%%%%%
    \specialrule{0em}{0ex}{0ex}
    \multicolumn{1}{c}{\small \textbf{Response Time -- in seconds: Study~1}} \\
   \specialrule{0em}{0ex}{2ex}
    \multirow{1}{*}{\includegraphics[height=\meanfigheight]{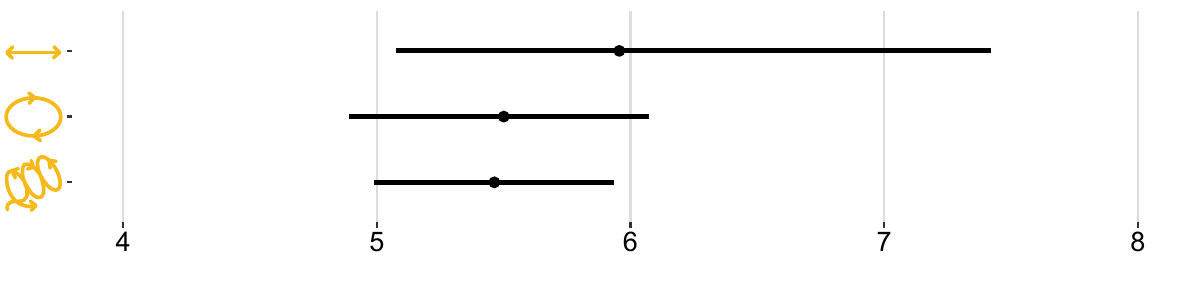}}&%Image: Alpha mean
    5.96,&% mean alpha - line
    [5.07,7.42]% CI alpha - line
    \\
    %% row 1.2 
    &%image row stays empty
    5.50&% mean alpha - circular
    [4.89,6.07]% CI alpha - circular
    %image row stays empty
    \\
    %% row 1.3
    &%image row stays empty
    5.46&% mean alpha - cones
    [4.99,5.93]% CI alpha - cones
    %image row stays empty
    \\ 
    \specialrule{0em}{0ex}{2ex}
    %% subfigures title
    \multicolumn{1}{c}{\fontsize{7}{7}\selectfont Means with CIs}\\ 
    \specialrule{0em}{0ex}{2ex}
    \multirow{1}{*}{\includegraphics[height=\meanfigheight]{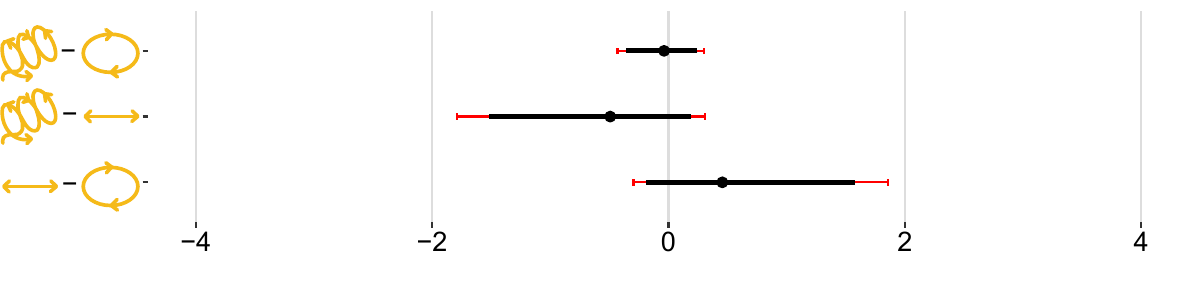}}&%Image: Beta mean
    -0.04&% mean beta - line
    [-0.43,0.30]% CI beta - line
    \\
    &
    -0.49&% mean beta - circular
    [-1.79,0.31]% CI beta - circular
    \\
    &
    0.46&% mean beta - cones
    [-0.30,1.86]% CI beta - cones
    \\ 
    \specialrule{0em}{0ex}{2ex}
    \multicolumn{1}{c}{\fontsize{7}{7}\selectfont Pairwise differences with CIs}\\
    %%%%%%%% Title row: response time %%%%%%
    \cline{1-3}
    %%%%%%%% Title row: fitness data Accuracy %%%%%%
    \specialrule{0em}{0ex}{2ex}
    \multicolumn{1}{c}{\small \textbf{Fitness Data Comparison Accuracy -- in percent: Study~1}} \\
    \specialrule{0em}{0ex}{2ex}
    \multirow{1}{*}{\includegraphics[height=\meanfigheight]{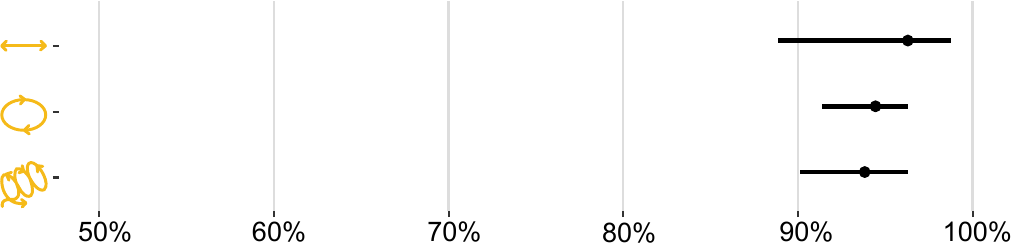}}&%Image: Alpha mean 
    96.3&% mean alpha - line
    [88.9,98.8]\\% CI alpha - line
   
    %% row 1.2 
    &%image row stays empty
    94.4&% mean alpha - circular
    [91.4,96.3]\\% CI alpha - circular
   
    %% row 1.3
    &%image row stays empty
    93.8&% mean alpha - cones
    [90.1,96.3]\\% CI alpha - cones
    \specialrule{0em}{0ex}{4ex}
    %% subfigures title
    \multicolumn{1}{c}{\fontsize{7}{7}\selectfont Means with CIs}\\
    \specialrule{0em}{0ex}{2ex}
    
    \multirow{1}{*}{\includegraphics[height=\meanfigheight]{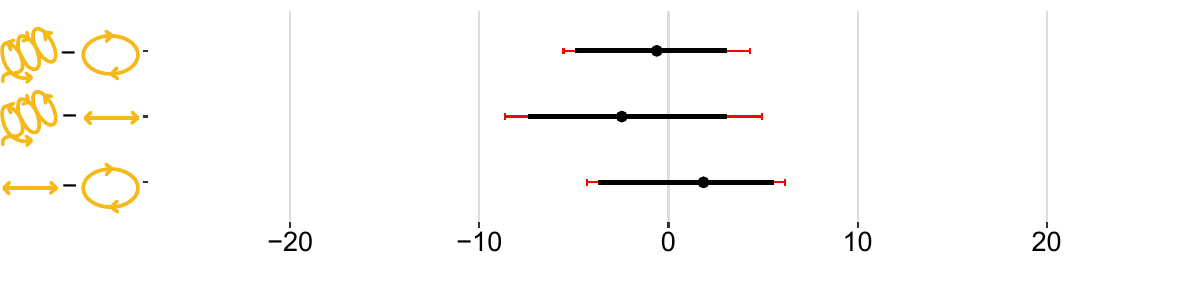}}&%Image: Beta mean
    -0.6&% mean beta - line
    [-5.6,4.3]% CI beta - line
    \\
    &%image row stays empty
    -2.5&% mean beta - circular
    [-8.6,4.9]% CI beta - circular
    \\
    &%image row stays empty
    1.9&% mean beta - cones
    [-4.3,6.2]% CI beta - cones
    \\
    \specialrule{0em}{0ex}{2ex}
    %% subfigures title
    \multicolumn{1}{c}{\fontsize{7}{7}\selectfont Pairwise differences with CIs} \\
    \specialrule{0em}{0ex}{2ex}
    %%%%%%%% Title row: Fitness Data Accuracy %%%%%%
    \cline{1-3}
    %%%%%%%% Title row: Answer Accuracy %%%%%%
    \specialrule{0em}{0ex}{2ex}
    \multicolumn{1}{c}{\small \textbf{Proportion Estimation Accuracy -- in percent: Study~1}} \\
    \specialrule{0em}{0ex}{2ex}
    \multirow{1}{*}{\includegraphics[height=\meanfigheight]{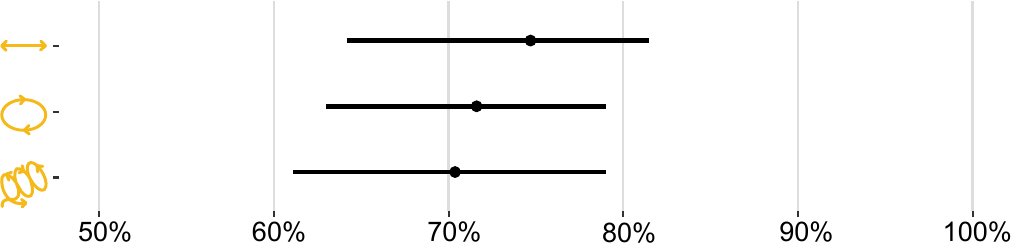}}%Image: Alpha mean
    &74.7% mean alpha - line
    &[64.2,81.5]% CI alpha - line
    \\
    %% row 1.2 
    &%image row stays empty
    71.6&% mean alpha - circular
    [63.0,79.0]% CI alpha - circular
    \\
    %% row 1.3
    &%image row stays empty
    70.4&% mean alpha - cones
    [61.1,79.0]% CI alpha - cones
    \\
    \specialrule{0em}{0ex}{4ex}
    %% subfigures title
    \multicolumn{1}{c}{\fontsize{7}{7}\selectfont Means with CIs}
    \\
    \specialrule{0em}{0ex}{2ex}
    \multirow{1}{*}{\includegraphics[height=\meanfigheight]{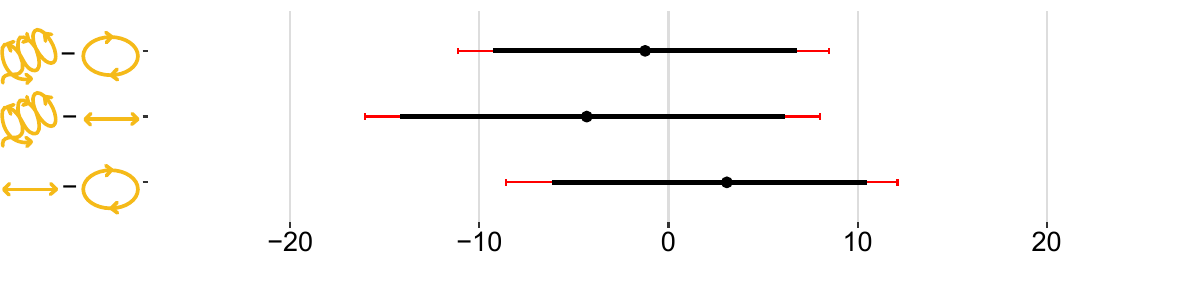}}&%Image: Beta mean
    -1.2,&% mean beta - line
    [-11.1,8.5]% CI beta - line
    \\
    &%image row stays empty
    -4.3&% mean beta - circular
    [-16.0,8.0]% CI beta - circular
    \\
    &%image row stays empty
    3.1&% mean beta - cones
    [-8.6,12.1]% CI beta - cones
    \\
    \specialrule{0em}{0ex}{2ex}
    \multicolumn{1}{c}{\fontsize{7}{7}\selectfont Pairwise differences with CIs} \\
    \specialrule{0em}{0ex}{2ex}
    %%%%%%%% Title row:  Answer Accuracy %%%%%%
    %\specialrule{0em}{4ex}{5ex}
    %\cline{1-3}
     
    \end{tabular}

    \vspace{-0.6cm}
\end{table*}
